# Supplementary material for: ToM: Leveraging Tree-oriented MapReduce for Long-Context Reasoning in Large Language Models
Source: arXiv:2511.00489 source file (2025-11-01)
Supplement: Supplementary file 1 [file appendix_copy.tex]

\newpage
\section*{Appendix}
This appendix provides supplementary information and further analysis of the ToM framework. We begin by presenting performance results for ToM on additional long-context question answering tasks, extending the evaluations in the main paper. This is followed by a detailed examination of ToM's computational complexity, assessing both the overhead of DocTree construction and the efficiency of its reasoning process. We also discuss key methodological considerations, such as the implications of information loss during document compression in ToM, and briefly address the quality of the hierarchical semantic parser. Finally, we offer an in-depth comparison with traditional Retrieval-Augmented Generation (RAG) methods, further highlighting the architectural and performance advantages of ToM's tree-oriented approach.

\subsection*{Performance on Additional Tasks}

In addition to HQA, 2Wiki, MuSi, Inf.QA, and Inf.MC, we also evaluated ToM on additional QA tasks: the Long In-context Learning task—User Guide QA and the Long-dialogue History Understanding task—Dialogue History QA. The experimental results in Table~\ref{additional tasks} demonstrate that on User Guide QA, our ToM approach achieved an accuracy of 65.0\%, outperforming the baseline GPT-4o model by 12.5 percentage points (from 52.5\%) and GPT-4o+LongAgent by 5.0 percentage points (from 60.0\%). Similarly, on Dialogue History QA, ToM reached 68.4\% accuracy, surpassing the baseline GPT-4o by 15.8 percentage points (from 52.6\%) and GPT-4o+LongAgent by 5.2 percentage points (from 63.2\%).

\begin{table}[!h]
\centering  
\small
\resizebox{\columnwidth}{!}{%
\begin{tabular}{lcc}
\toprule
\textbf{} & \textbf{User Guide QA}  & \textbf{Dialogue History QA} \\
\midrule
GPT-4o & 52.5 & 52.6 \\
+ LongAgent & 60.0 & 63.2 \\
+ ToM & \textbf{65.0} & \textbf{68.4} \\
\bottomrule
\end{tabular}
}
\vspace{-7pt}
\caption{Accuracy on User Guide QA and Dialogue History QA.}
\label{additional tasks}
\end{table}


These statistically significant and consistent performance improvements across diverse long-context tasks provide empirical evidence for ToM's robust generalizability. The observed enhancements can be attributed to the fundamental architectural advantages of our framework: specifically, the tree-oriented MapReduce methodology enables hierarchical document structuring through semantic parsing and bottom-up aggregation, preserving critical semantic relationships that would otherwise be lost in traditional approaches. Unlike conventional RAG methods that rely on sequential reasoning or divide-and-conquer frameworks that process chunks in isolation, ToM's recursive reasoning mechanism explicitly maintains parent-child relationships between document segments and facilitates long-range information flow across the entire DocTree. This structural coherence is particularly beneficial for dialogue-based tasks, as evidenced by the substantial 15.8 percentage point improvement on Dialogue History QA, where maintaining contextual continuity across multiple conversational turns is essential for accurate comprehension and reasoning. The experimental findings thus substantiate our hypothesis that tree-based reasoning offers a more effective paradigm for complex long-context understanding tasks that require sophisticated multi-hop inference capabilities.


\subsection*{Complexity Analysis}

When comparing our approach, ToM, to traditional methods like RAG or divide-and-conquer frameworks, one noticeable difference is the additional tree construction step that ToM incorporates. While this naturally leads to extra computational overhead, our experimental evaluations show that the added time is justified by the significant improvements in performance. The construction of the DocTree in ToM consists of three distinct steps: 1) embedding \textbf{chunks before constructing}, which involves processing document chunks to obtain their respective embeddings; 2) \textbf{Inferencing during hierarchical semantic parsing}, where the chunk's textual content is parsed into a structured, hierarchical representation, capturing the internal relationships between different segments within the chunk; and 3) \textbf{bottom-up summarizing}, where these subtrees are aggregated to form the complete DocTree. Each of these steps is crucial for achieving the hierarchical structure that enables effective long-context reasoning.

\begin{table}[!h]
\centering
\small
\begin{tabular}{lccccc}
\toprule
\textbf{Time} & \textbf{10k} & \textbf{80k} & \textbf{120k} & \textbf{250k} \\
\midrule
Embedding & 0.6 & 1.9 & 2.7 & 5.3  \\
Inference & 9.9 & 29.4 & 34.3 & 37.2  \\
Summarization & 8.0 & 27.0 & 28.1  & 32.9  \\
Total  & 18.5 & 58.3 & 65.1 & 75.4  \\
\bottomrule
\end{tabular}

\caption{Average constructing time (s) on varying lengths.}
\label{tab:constructing time}
\end{table}


\vspace{-10pt}
\begin{table}[!h]
\centering
\small
\begin{tabular}{lcccc}
\toprule
 & \textbf{RAG} & \textbf{LongAgent} & \textbf{Our ToM} \\
\midrule
Time & 5.4 & 236.8 & 145.0 \\
\bottomrule
\end{tabular}
\caption{Average time cost on Inf.QA over 100k tokens.}
\label{tab:reasoning time}
\end{table}


From the experimental results shown in Tab~\ref{tab:constructing time}, it is clear that the construction time increases with document length, which is expected due to the additional tree-building step. The total time required for constructing the DocTree increases steadily as the document length grows, with processing times of 18.5 seconds for 10k tokens, 58.3 seconds for 80k tokens, and 75.4 seconds for 250k tokens. Although the construction time for ToM is higher than that of RAG and other divide-and-conquer methods, the time spent remains manageable and well-justified, particularly when considering the significant improvements in reasoning performance that ToM delivers. The added time investment in DocTree construction enables more comprehensive processing of long documents, leading to more accurate and coherent reasoning results.

Turning to the reasoning performance presented in Tab~\ref{tab:reasoning time}, the results further illustrate the effectiveness of ToM. While RAG and LongAgent show promising performance in shorter contexts, they struggle to maintain efficiency and accuracy when processing ultra-long documents. ToM, in contrast, achieves significantly better performance with reasoning times of 145.0 seconds for 100k tokens, outperforming both RAG (5.4 seconds) and LongAgent (236.8 seconds). This demonstrates that, despite its longer reasoning time, ToM achieves a better balance between efficiency and effectiveness. By leveraging its hierarchical structure and recursive MapReduce reasoning, ToM excels in integrating information across long contexts, providing more accurate and reliable reasoning results. Therefore, while ToM does require more time for both construction and reasoning, the performance improvements it offers make this additional time expenditure highly beneficial and worthwhile.

\subsection*{Quality of the Hierarchical Semantic Parser}
Current LLMs can perform stable parsing without tuning and can achieve better performance after distillation (loss in Figure~\ref{fig:loss}, with no matching failures during thousands of parsing instances.
\begin{figure}[!t]
    \centering
    \includegraphics[width=0.9\linewidth]{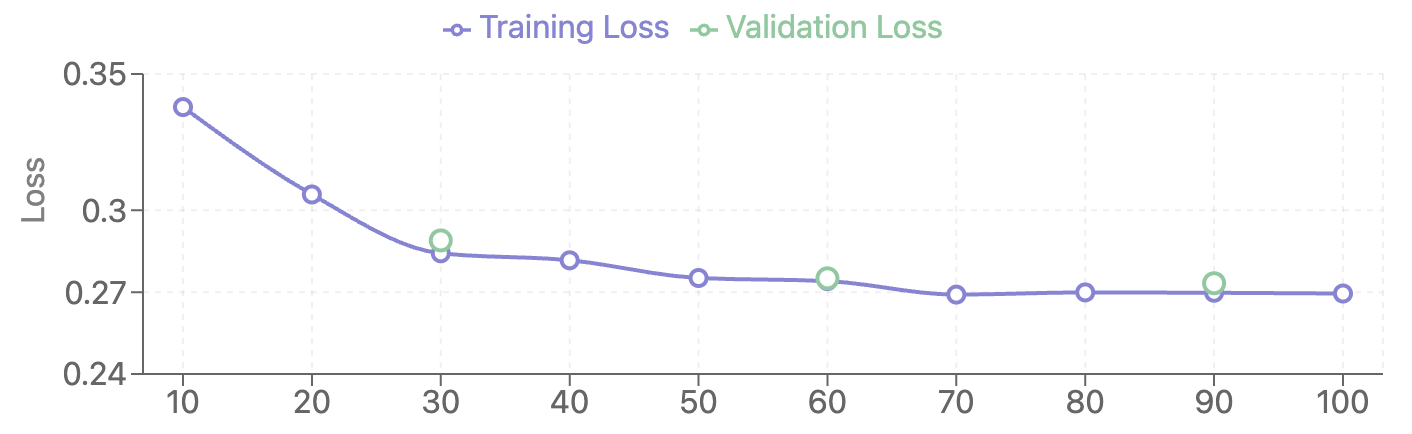}
    \caption{Loss curves of the HSP using the Qwen2.5-3B-Instruct.}
    \label{fig:loss}
\end{figure}

\subsection*{DocTree Compression}
\begin{algorithm}[!b]
\hrule
\vspace{1.5mm}\textbf{\small Algorithm 2: Query-Aware DocTree Compression}
\label{Alg:compression}
\vspace{1.5mm}
\hrule
\small
\fontsize{8}{10}\selectfont
\SetAlgoLined
\DontPrintSemicolon
\SetAlgoVlined
\SetAlgoSkip{1.5mm}  % 统一调整行距
\vspace{3mm}
\KwIn{Long context \( C \), Query \( q \), Retriever \( \mathcal{R} \), Selection scale \( k \)}
\KwOut{Compressed set of chunks \( \{c'_1, c'_2, \dots, c'_k\} \)}

\BlankLine
\textbf{Step 1: Embedding Generation} \;
Generate query embedding \( e_q \) for \( q \) using \( \mathcal{R} \)\;
Split \( C \) into fixed-length token chunks \( \{c_1, c_2, \dots, c_n\} \)\;
\ForEach{chunk \( c_i \)}{
    Generate embedding \( e_{c_i} \) for \( c_i \) using \( \mathcal{R} \)\;
    Compute cosine similarity \( \text{Sim}(e_{c_i}, e_q) \) for \( e_{c_i} \) and \( e_q \)\;
}

\BlankLine
\textbf{Step 2: Chunk Selection} \;
Select the top-\( k \) chunks based on similarity scores:
\[
\{c'_1, c'_2, \dots, c'_k\} = \text{TopKSim}(q, \{c_1, c_2, \dots, c_n\})
\]

\BlankLine
\textbf{Step 3: Build Compressed DocTree \( \mathcal{T} \) using \(\{c'_1, c'_2, \dots, c'_k\}\)}

\BlankLine
\textbf{Return:} Compressed DocTree \( \mathcal{T} \) aligned with query \( q \)\;
\vspace{2mm}
\hrule
\end{algorithm}

\subsection*{Information Loss during Compression}

Our DocTree compression strategy, which employs query-aware top-k selection using embeddings, does introduce a deliberate tradeoff between computational efficiency and information completeness. By selectively focusing on the most relevant chunks for DocTree construction, we reduce processing time while maintaining high performance on most reasoning tasks. However, this process may potentially exclude intermediate information that could be valuable for capturing certain long-range dependencies, particularly in cases requiring complex multi-hop reasoning across seemingly unrelated document sections.

To address this concern, we emphasize the flexible nature of our framework, which allows practitioners to adjust the compression parameters based on their specific requirements. For applications prioritizing maximum reasoning accuracy where computational resources are less constrained, compression can be made optional, permitting the construction of complete DocTrees that preserve all document information. 

Our experiments with varying compression levels indicate that increasing the number of selected chunks generally improves performance, with diminishing returns beyond a certain threshold. This suggests that while some information loss occurs during compression, our embedding-based selection effectively identifies most critical chunks, and the hierarchical structure of DocTree helps mitigate the impact of missing intermediate information by establishing connections between distant but semantically related chunks during the bottom-up aggregation process.


\subsection*{Compared to RAG}
ToM demonstrates superior performance across all benchmarks as evidenced by our experimental results. An intriguing aspect of this comparison is that ToM initially employs retrieval mechanisms similar to those in RAG for chunk selection, yet achieves significantly better outcomes in downstream reasoning tasks.

Retrieval-Augmented Generation (RAG) approaches have made significant contributions to question answering tasks by effectively enhancing recall—successfully retrieving chunks containing potentially relevant information. However, QA tasks inherently demand high precision in utilizing retrieved information to generate accurate answers. While RAG excels at gathering diverse relevant content, its flat concatenation of retrieved chunks and single-pass reasoning process presents challenges for complex queries requiring nuanced information integration.

Our Tree-oriented MapReduce (ToM) framework builds upon RAG's strong retrieval foundation while addressing this precision challenge through hierarchical processing. By organizing the same retrieved chunks into a structured DocTree, ToM enables a two-phase reasoning process that systematically improves precision. In the Map phase, ToM conducts fine-grained reasoning on individual sibling nodes in parallel, generating detailed rationales that capture essential supporting facts from each document segment. The subsequent Reduce phase then systematically aggregates these rationales across sibling nodes, resolving conflicts and reaching consensus at parent nodes.
This recursive process enables ToM to progressively refine understanding from leaf nodes to root nodes, preserving context coherence throughout the document hierarchy. By facilitating information flow between parent-child relationships and across sibling nodes, ToM transforms high-recall retrieved content into high-precision answers, particularly excelling at complex queries requiring integration of distributed information and resolution of apparent contradictions.

\begin{figure*}[!t]
    \centering
    \includegraphics[width=\textwidth, height=\textheight, keepaspectratio]{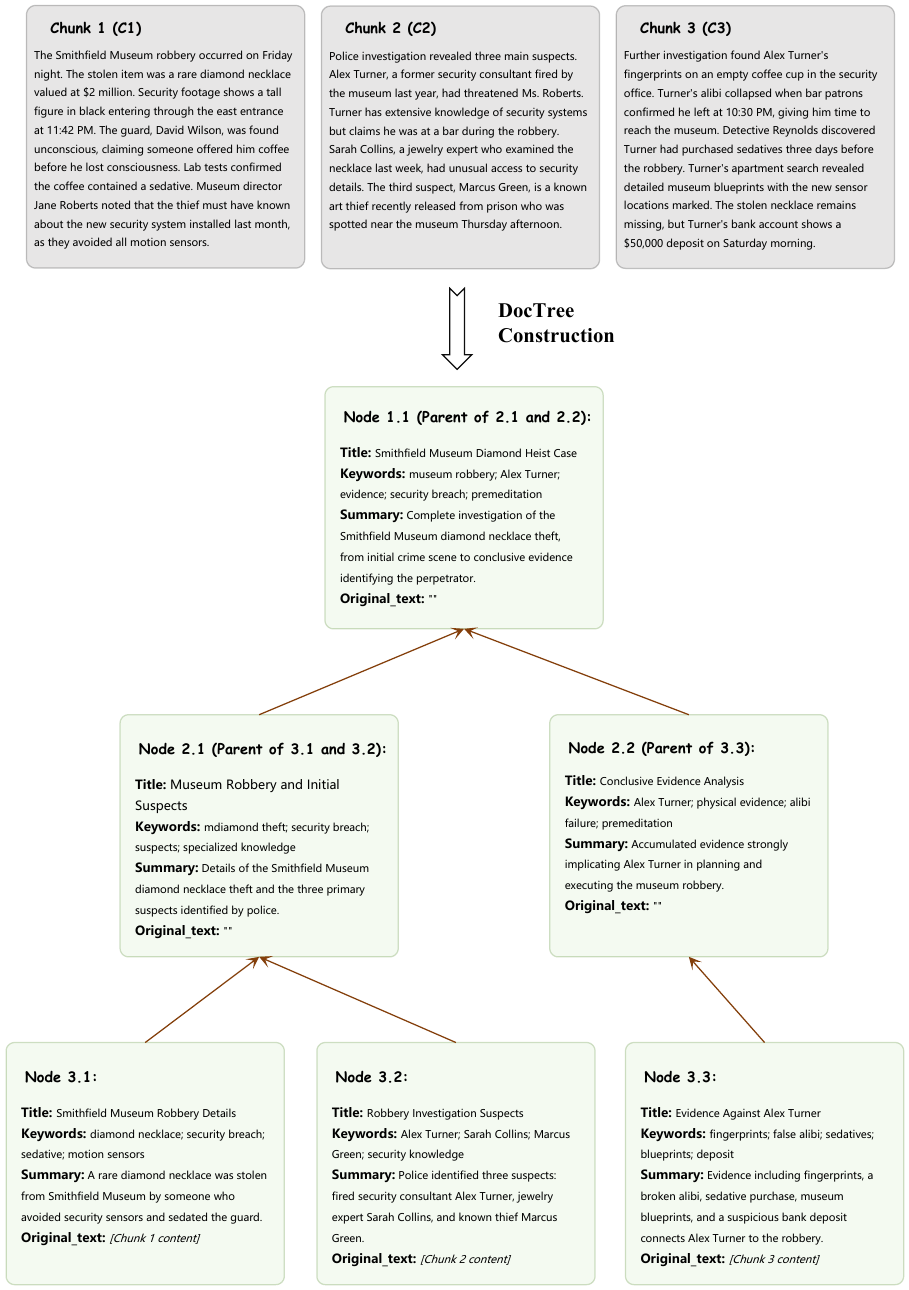}
    % \vspace{5pt}
    \caption{DocTree construction case.}
\end{figure*}

\begin{figure*}[!t]
    \centering
    \includegraphics[width=\textwidth, height=\textheight, keepaspectratio]{Figures/case_reasoning(1).pdf}
    \caption{MapReduce reasoning case.}
\end{figure*}


\begin{figure*}[!t]
    \centering
    \includegraphics[width=0.8\linewidth]{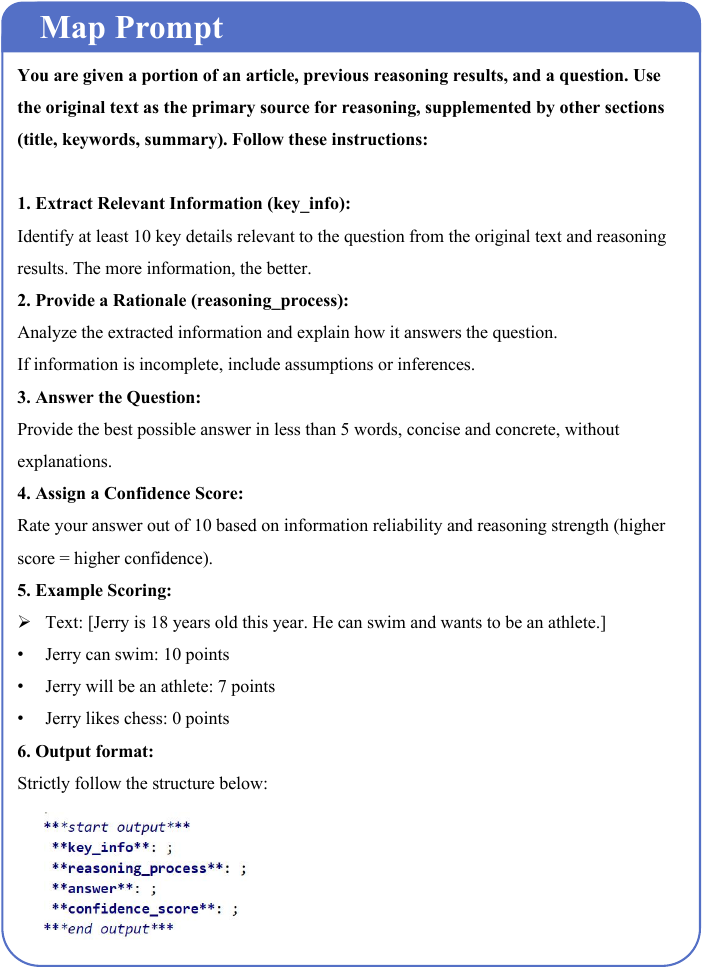}
    \caption{Prompt for Map step.}
\end{figure*}

\begin{figure*}[!t]
    \centering
    \includegraphics[width=0.8\linewidth]{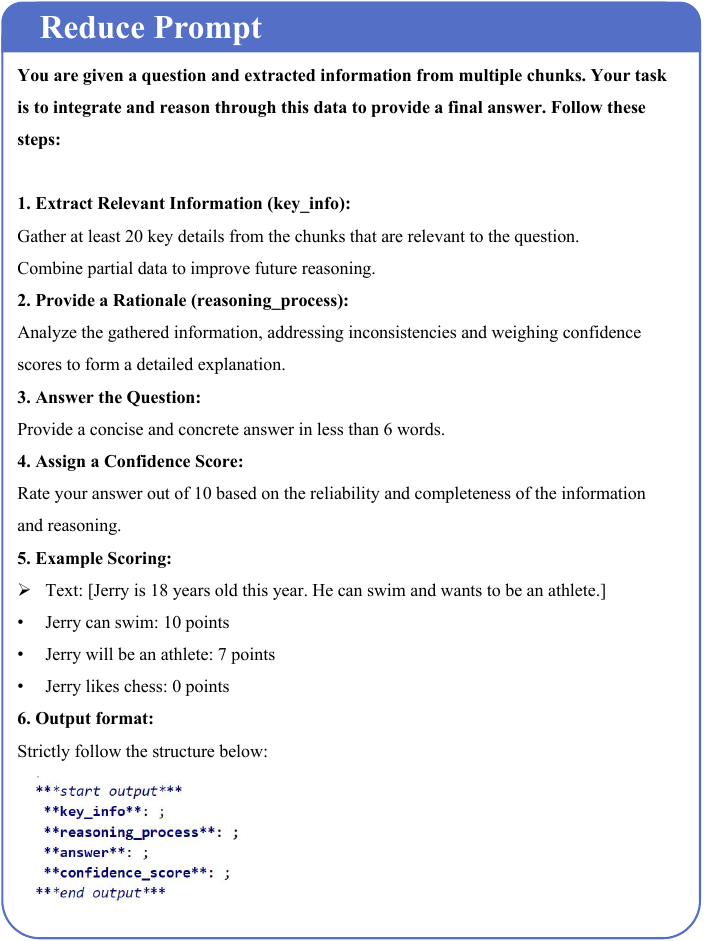}
    \caption{Prompt for Reduce step.}
\end{figure*}


\begin{figure*}[!t]
    \centering
    \includegraphics[width=0.8\linewidth]{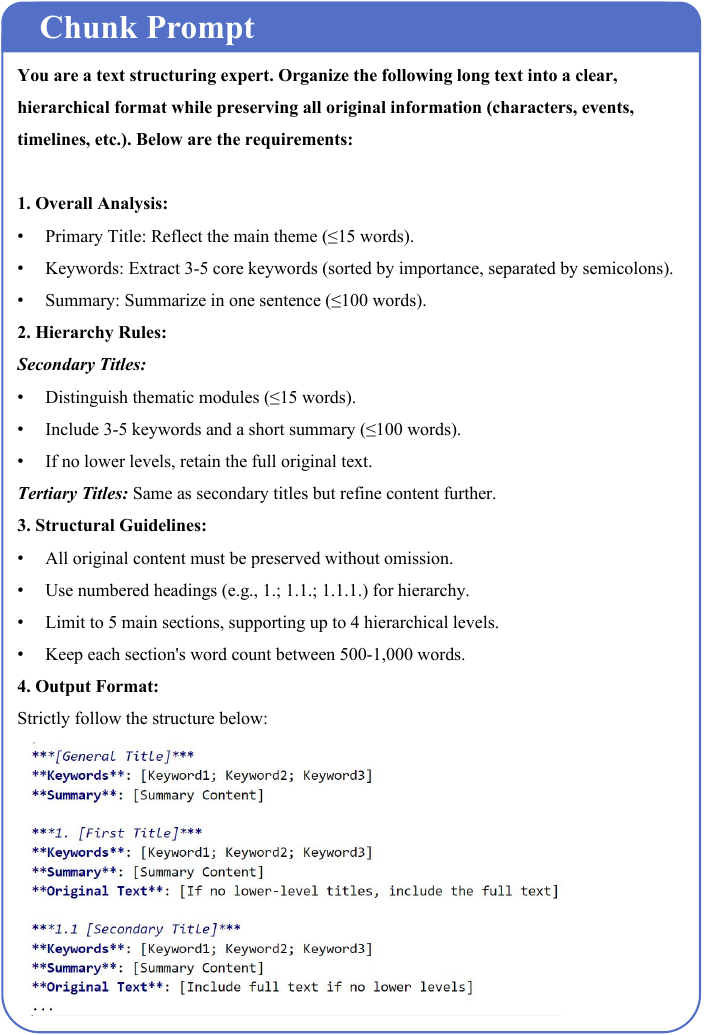}
    \caption{Prompt for Hierarchical Semantic Parsing.}
\end{figure*}
